# Supplementary material for: Suppressed Auger scattering and tunable light emission of Landau-quantized massless Kane electrons
Source: arXiv:1906.10905 source file (2020-07-21)
Supplement: Supplementary file 1 [file SI.pdf]

# Suppressed Auger scattering and tunable light emission of Landau-quantized massless Kane electrons – *Supplementary materials*

D. B. But,[1,2] M. Mittendorff,[3,4] C. Consejo,[1] F. Teppe,[1] N. N. Mikhailov,[5] S. A. Dvoretskii,[5] C. Faugeras,[6] S. Winnerl,[3] M. Helm,[3] W. Knap,[1,2] M. Potemski,[6,7] and M. Orlita[6,8]

[1] *Laboratoire Charles Coulomb, UMR CNRS 5221, University of Montpellier, Montpellier 34095, France*
[2] *CENTERA laboratories, Institute of High Pressure Physics, Polish Academy of Sciences, 01-142 Warsaw, Poland*
[3] *Helmholtz-Zentrum Dresden-Rossendorf, PO Box 510119, 01314 Dresden, Germany*
[4] *Universität Duisburg-Essen, Fakultät für Physik, 47057 Duisburg, Germany*
[5] *A.V. Rzhanov Institute of Semiconductor Physics, Siberian Branch, Russian Academy of Sciences, Novosibirsk 630090, Russia*
[6] *Laboratoire National des Champs Magnétiques Intenses, CNRS-UGA-UPS-INSA-EMFL, 25 rue des Martyrs, 38042 Grenoble, France*
[7] *Faculty of Physics, Institute of Experimental Physics, University of Warsaw, ul. Pasteura 5, 02-093 Warszawa, Poland*
[8] *Charles University, Faculty of Mathematics and Physics, Ke Karlovu 5, 121 16 Prague 2, Czech Republic*

In these Supplementary materials we provide readers with additional experimental data and also discuss possible ways of electrical and optical pumping of massless Kane electrons, which may allow one to achieve population inversion necessary for laser operation.

## CYCLOTRON EMISSION FROM HGCDTE SAMPLES WITH NON-ZERO ENERGY BAND GAP

To crosscheck the results of cyclotron emission experiments performed on the $Hg_{1-x}Cd_xTe$ sample with a vanishing band gap ($x = 0.17$), other two MBE-grown samples have been prepared and studied. These had an identical layer sequence, but the cadmium concentration in the 3.2-micron-thick active region has been increased to $x = 0.19$ and 0.23. This translates into the energy band gap of $E_g \approx 45$ and 120 meV [1], respectively. Even though cyclotron emission is weaker in these gapped samples, it can still be observed, in line with earlier studies [2]. The experimentally deduced spectral positions of cyclotron emission maxima have been plotted in Fig. S1 and compared with expectations of a simple theoretical model (solid lines), the description of which follows.

The conduction-band spectrum of Landau levels for (massive) Kane electrons with the (positive) energy band gap $E_g$ reads [3, 4]:

$$E^K_{N,\sigma}(k) = \sqrt{(E_g/2)^2 + 2e\hbar B(N - 1/2 \pm \sigma/2) + v^2\hbar^2k^2}. \tag{S1}$$

Cyclotron emission modes are electric-dipole-active transitions $N \to N-1$ ($N = 1, 2, 3\ldots$) with the spin index $\sigma$ preserved. A dominant contribution to the cyclotron emission comes from the bottom of LLs ($k \approx 0$), where maxima in the (joint) density of states appear. The energies of cyclotron modes thus may be expressed as: $E^K_{N+1}(0) - E^K_N(0)$. To compare theoretical expectations with the experimental data, the energies of two cyclotron emission modes with the final state of electrons in two lowest conduction-band LLs ($N = 1$ for $\sigma = -1/2$ and $1/2$) have been plotted in Fig. S1 as a function of the magnetic field applied to the sample. These curves were calculated for the expected size of $E_g$ [1] and using the velocity parameter typical of Kane electrons in HgCdTe, $v = 1.06 \times 10^6$ m/s, see Refs. [3, 5]. Very good agreement between experimental data and theory corroborates the interpretation of the observed emission spectra in terms of cyclotron emission.

To compare the emission intensity from gapped samples with the one observed from the gapless specimen, we performed a cyclotron emission experiment in which the signals from the gapless ($x = 0.17$) and small-gap ($x = 0.19$) samples were collected during the same run, see Fig. S2. To put these results into the right context, let us note that these emission experiments were performed in the standard configuration [2], *i.e.*, with relatively weak electrical pumping. Such pumping establishes approximately Boltzmann-like distribution of conduction-band electrons among Landau levels. Therefore, there is only a relatively low electron density in the excited LLs, typically $10^{11}$ cm$^{-3}$ as compared to the total electron density of $10^{13} - 10^{14}$ cm$^{-3}$ [6]. At such low densities of excited electrons, inter-LL Auger scattering rate ($\tau^{-1} \propto n$) is expected to be still comparable with the one due to other non-radiative channels

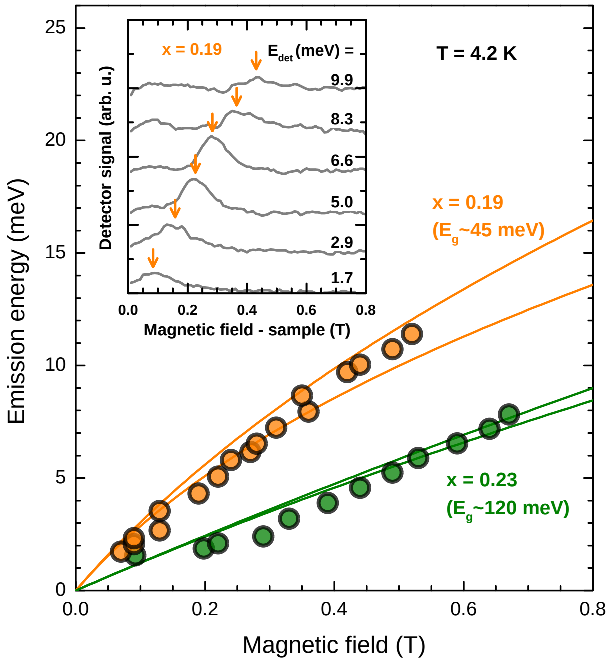


Figure S1. Cyclotron energies as a function of the magnetic field applied to the sample measured on $Hg_{1-x}Cd_xTe$ samples with the cadmium content of $x = 0.19$ and 0.23, which correspond to energy band gaps of $E_g \approx 45$ and 120 meV, respectively. The solid lines show the energies of two cyclotron emission modes with the final states of electrons in the lowest two LLs ($N = 1$, $\sigma = 1/2$ and $N = 1$, $\sigma = -1/2$). Inset: the cyclotron emission traces for the $Hg_{0.81}Cd_{19}Te$ measured as a function of the magnetic field applied to the sample. The vertically stacked traces correspond to selected resonant absorption energies $E_{\mathrm{det}}$ in the InSb detector (tuned by the magnetic field applied to the detector).

(mainly emission of phonons) [6]. Hence, there is no reason to expect some enormous enhancement of cyclotron emission when only one from non-radiative channels is switched off. The observed difference in the emission intensity, which reaches roughly one order of magnitude (Fig. S2) between the gapped ($x = 0.19$) and gapless ($x = 0.17$) samples, thus indeed indicates significant suppression of Auger recombination (while other non-radiative channels remain active). The effect of suppressed Auger scattering should play a profound role under strong electrical or optical pumping conditions. It should allow one to establish a considerable population inversion, which cannot be created in parabolically dispersing systems with an equidistant set of LLs. Let us now discuss the ways how such an inversion could be built up.

## MASSLESS KANE ELECTRONS – PUMPING SCHEMES

Electrical and optical pumping belong to the most common ways of achieving the population inversion $\Delta n$ in active media of lasers. Here we sketch a simple pumping scheme, which may allow one to achieve the population inversion in gapless HgCdTe. We also append quantitative estimates of $\Delta n$. We propose to pump HgCdTe either optically, using non-resonant monochromatic radiation with the photon energy $E_{\mathrm{pump}} = \hbar\omega$, or electrically, by embedding bulk gapless HgCdTe in a $p$-$n$ junction created from HgCdTe with a non-zero band gap $E_g = E_{\mathrm{pump}}$ (for $x > 0.17$), as schematically plotted in Fig. S3.

As concluded in our pump-probe experiments, the optical injection of electrons into a Landau level at finite momentum states, $E^K_{N,\sigma}(k) \gg E^K_{N,\sigma}(0)$, results in their relatively fast relaxation towards $k \approx 0$ states of a given level. We assume that the number of injected electrons into the $n$-th LL roughly follows its density of states $\rho_N$ at the energy of $E_{\mathrm{pump}}$. Comparing the characteristic slopes of LLs (= dispersive Landau bands) at the fixed energy of $E_{\mathrm{pump}}$, see Fig. S3, we conclude that $\rho_{N+1} - \rho_N > 0$. This favors the creation of a population inversion between $N$-th and $N + 1$-th LL around $k \approx 0$.

Let us now estimate this inversion quantitatively. We will use the quantity $\Delta n/n$, which weights the population inversion by the total number of injected electrons into $N$-th and $N + 1$-th LLs: $\Delta n/n \approx (\rho_{N+1} - \rho_N)/\rho_N$. A straightforward calculation of the density of states implies, provided the pumping is well above the bottom of the

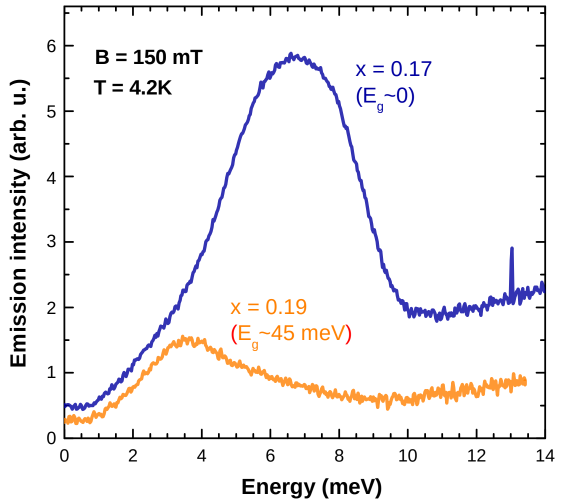


Figure S2. The cyclotron emission spectra measured in paralell on $Hg_{1-x}Cd_xTe$ samples with the cadmium concentration $x = 0.17$ and 0.19, which display the energy band gaps $E_g \approx 0$ and 45 meV, respectively. The back-ground-corrected integral emission from the gapless sample is by more than a factor of 5 larger as compared to the gapped sample.

given LL, $E_{\rm pump} > E^K_{N,\sigma}(0)$, the relative population inversion:

$$\frac{\Delta n}{n} \approx \frac{\hbar eB}{(E_{\rm pump}/v^2)} \cdot \frac{1}{E_{\rm pump}} \sqrt{1 - \left(\frac{E^K_N(0)}{E_{\rm pump}}\right)^2} \approx \frac{\hbar eB}{(E_{\rm pump}/v^2)} \cdot \frac{1}{E_{\rm pump}}. \tag{S2}$$

Interestingly, the relative population inversion $\Delta n/n$ becomes directly proportional to the classical cyclotron frequency of massless electrons at the energy of $E_{\rm pump}$: $\hbar eB/(E_{\rm pump}/v^2)$ [7, 8].

To get a numerical estimate, let us consider the pumping energy $E_{\rm pump} = 50$ meV and the characteristic magnetic field of $B = 100$ mT to obtain cyclotron emission in the THz range. This implies the relative population inversion $\Delta n/n$ better than $10^{-2}$ (higher values may be achieved by lowering $E_{\rm pump}$). In our pump-probe experiments, the total number of photo-generated electron by a single pulse reached $10^{16}$ cm$^{-3}$ without any clear contribution of fast Auger inter-LL scattering observed in the relaxation. In the estimated case, the injected electrons are distributed among a few lowest lying LLs ($N \leq 5$ for $B = 100$ mT and $E_{\rm pump} = 50$ meV), thus each with the characteristic density around $10^{14}$-$10^{15}$ cm$^{-3}$. This way, we obtain a population inversion above $10^{12}$-$10^{13}$ cm$^{-3}$ for several cyclotron modes between pairs of LLs with low indices. This is above the required value of $10^{12}$ cm$^{-3}$ estimated in the main text. Achieving measurable gain thus should be possible at least in the pulsed mode.


[1] Hansen, G.L., Schmit, J.L. & Casselman, T.N. Energy gap versus alloy composition and temperature in $Hg_{1-x}Cd_xTe$. *J. Appl. Phys.* **53**, 7099–7101 (1982).

[2] Gornik, E. Far infrared cyclotron emission in semiconductors. *J. Mag. Mag. Mater.* **11**, 39 – 46 (1979).

[3] Orlita, M. *et al.* Observation of three-dimensional massless Kane fermions in a zinc-blende crystal. *Nature Phys.* **10**, 233 (2014).

[4] Kacman, P. & Zawadzki, W. Spin magnetic moment and spin resonance of conduction electrons in $\alpha$-Sn-type semiconductors. *phys. stat. sol. (b)* **47**, 629–642 (1971).

[5] Teppe, F. *et al.* Temperature-driven massless Kane fermions in HgCdTe crystals: verification of universal velocity and rest-mass description. *Nature Comm.* **7**, 12576 (2016).

[6] Gornik, E. Landau emission in semiconductor. In Zawadzki, W. (ed.) *Narrow Gap Semiconductors. Physics and Applications. Lecture Notes in Physics*, vol. 133 (Springer, Berlin, 1980).

[7] Witowski, A.M. *et al.* Quasiclassical cyclotron resonance of dirac fermions in highly doped graphene. *Phys. Rev. B* **82**, 165305 (2010).

[8] Crassee, I. *et al.* Giant faraday rotation in single- and multilayer graphene. *Nature Phys.* **7**, 48 (2011).

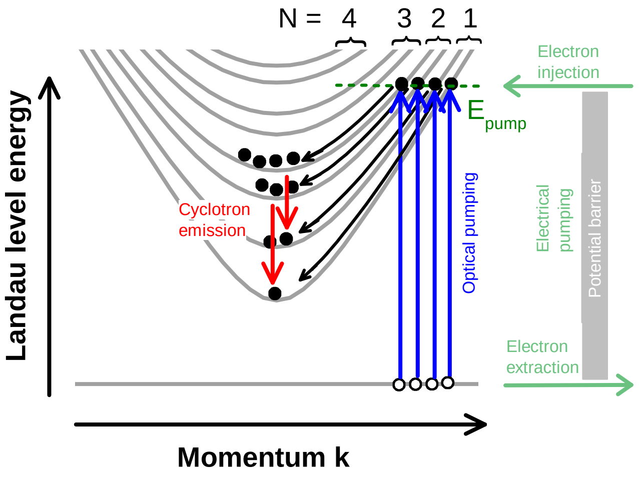


Figure S3. The LL spectrum of gapless HgCdTe with a schematic view of possible electrical and optical pumping, see the text.
